# Supplementary material for: Fundamental effective temperature measurements for eclipsing binary stars -- IV. Selection of new benchmark stars and first results for HD 22064
Source: arXiv:2303.15008 source file (2023-04-06)

# Fundamental effective temperature measurements for eclipsing binary stars - IV. Selection of new benchmark stars and first results for HD 22064.

Pierre F. L. Maxted

## Supplementary information

Light curves for all targets shown with best-fit models, and residuals from the best fit shown offset vertically in each panel. The best fits to 251 individual pairs of eclipses for TYC 8547-22-1 are all plotted together. The width of the two panels shown for each binary systems in phase units are equal so that the relative widths of the two eclipses can be seen directly.

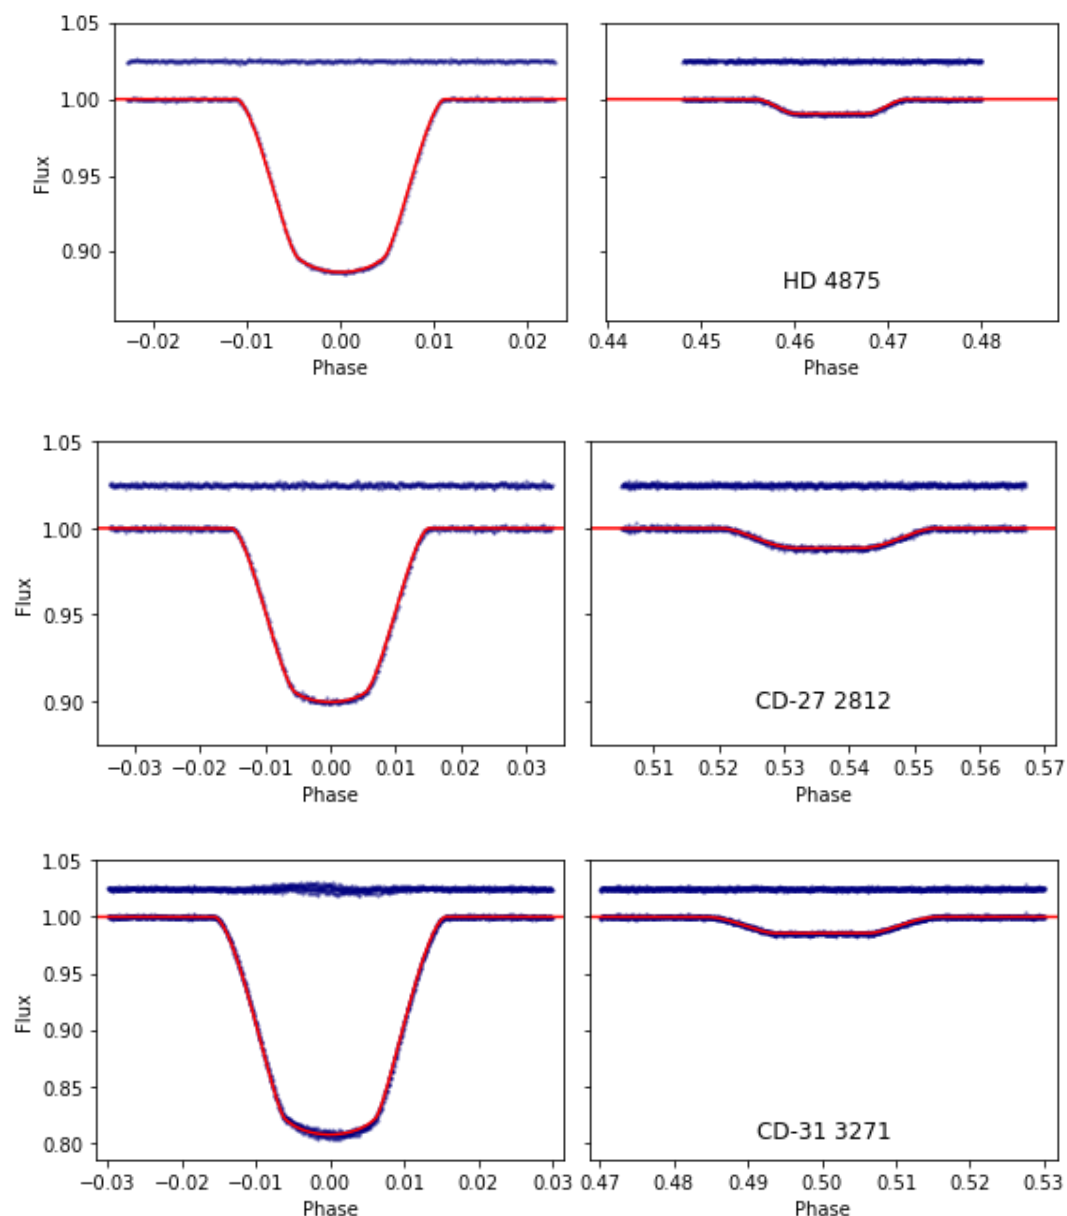

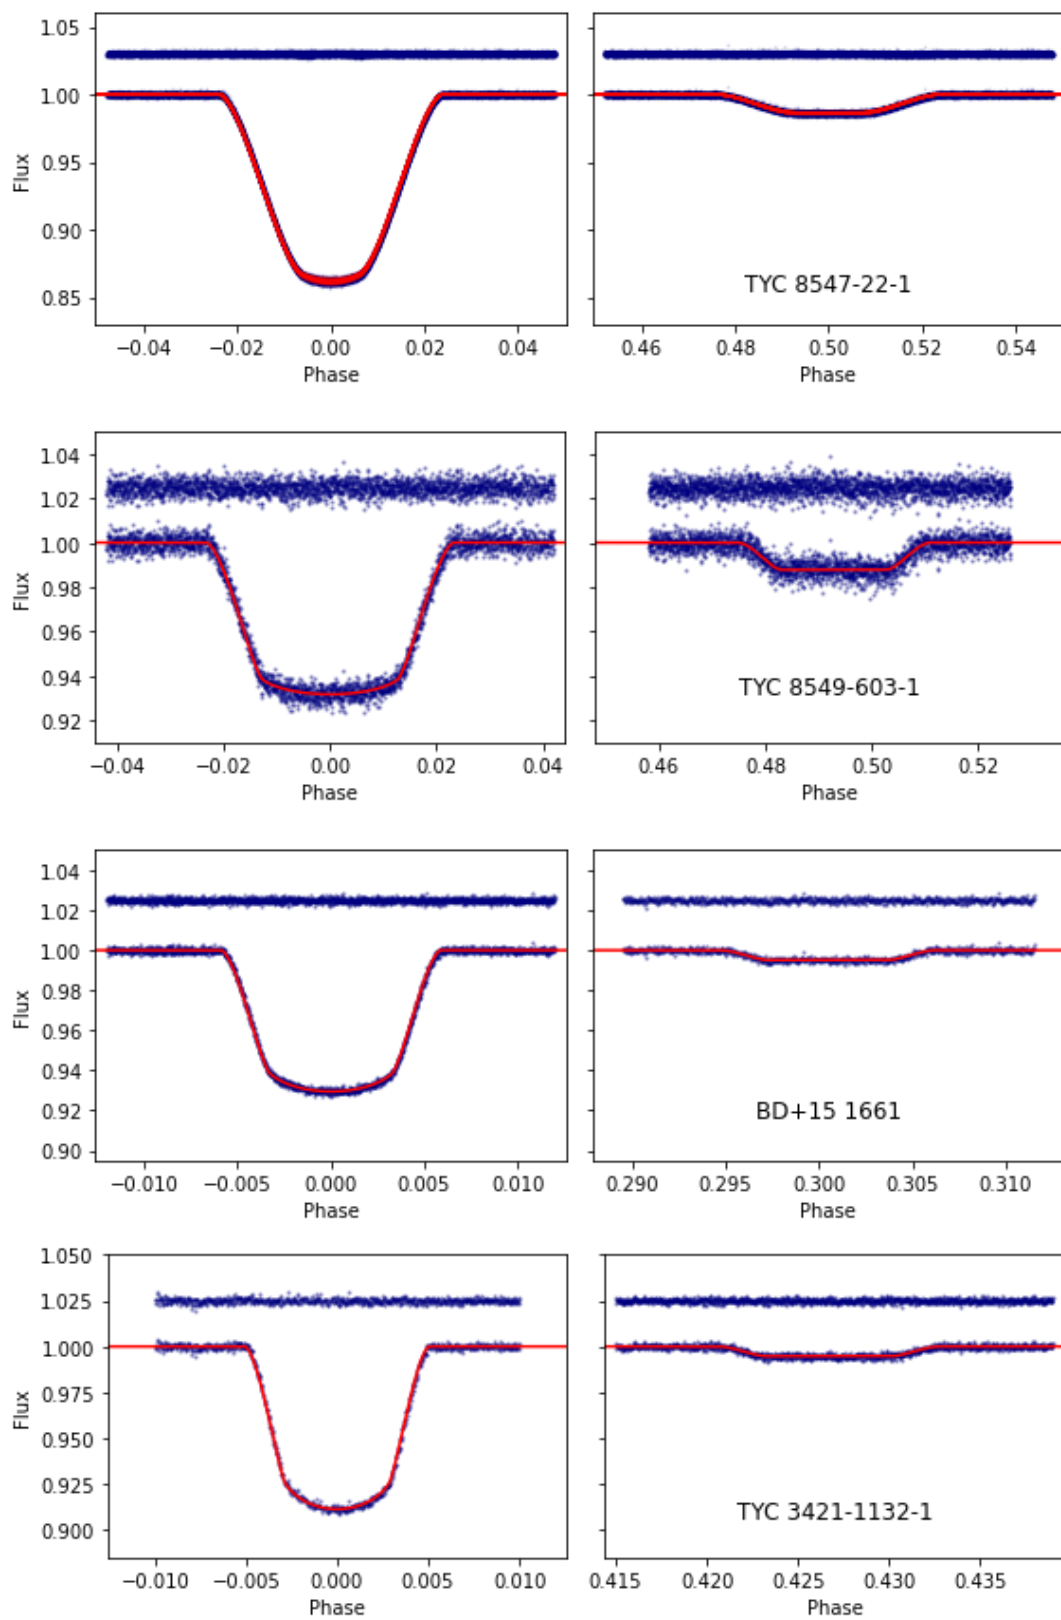

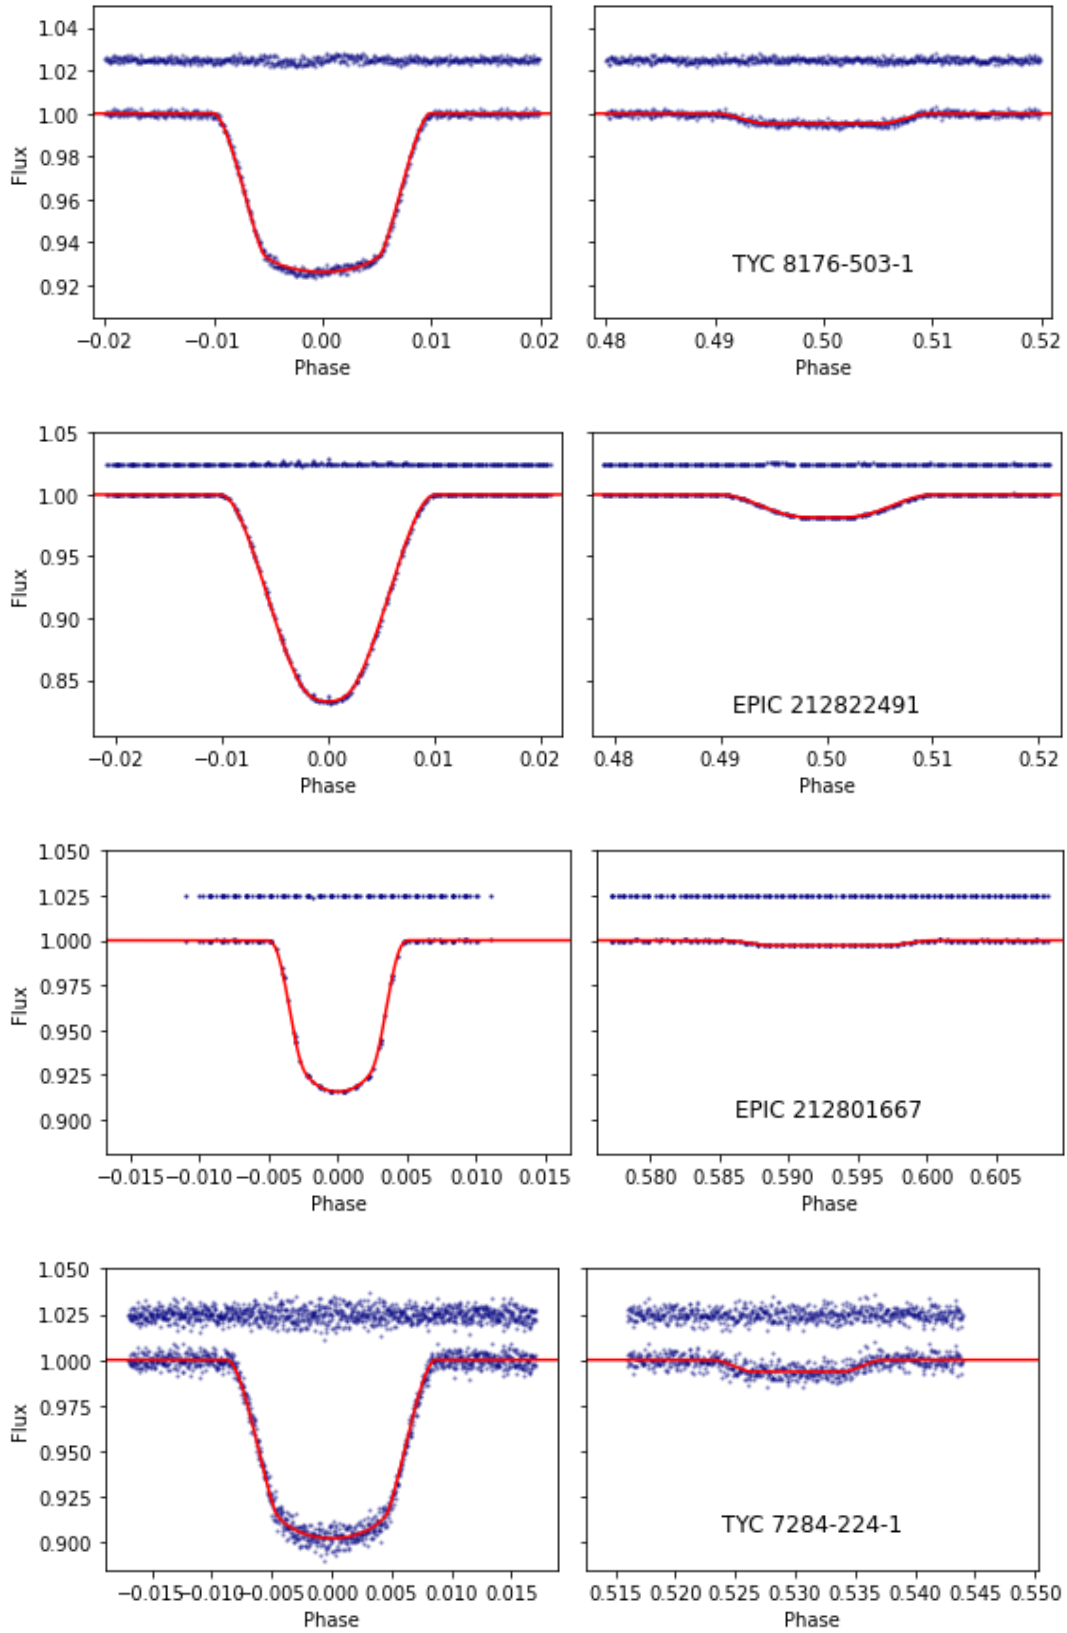

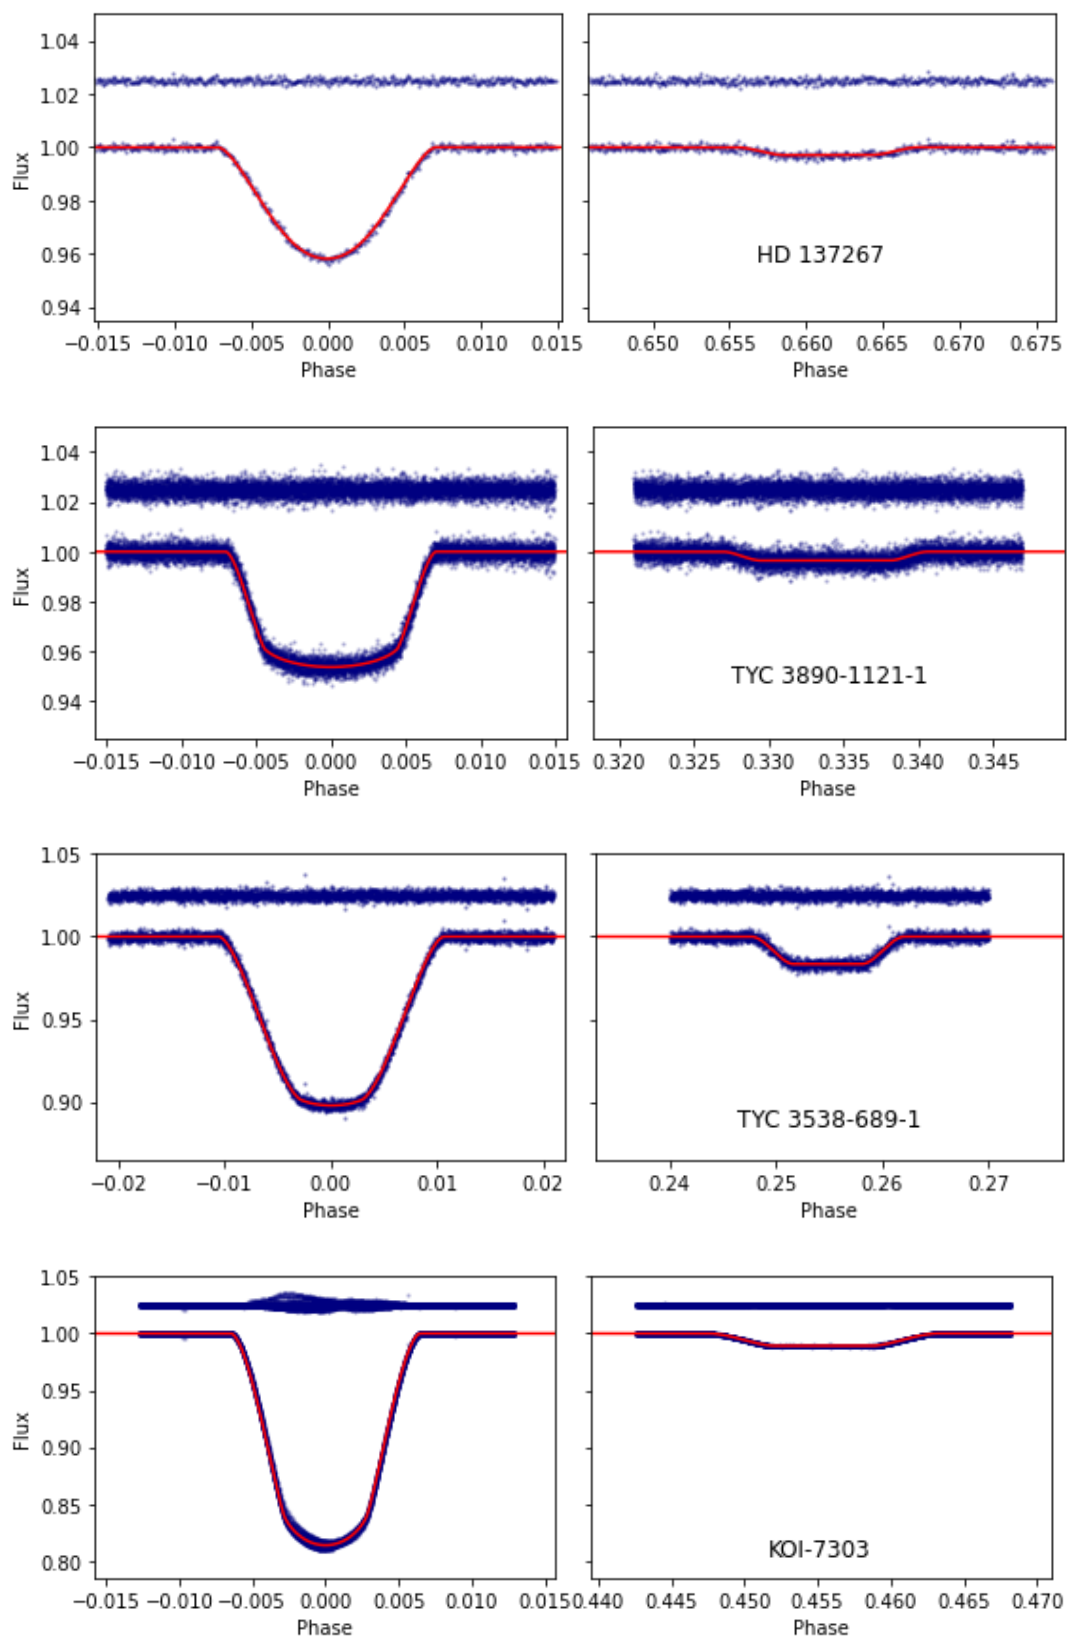

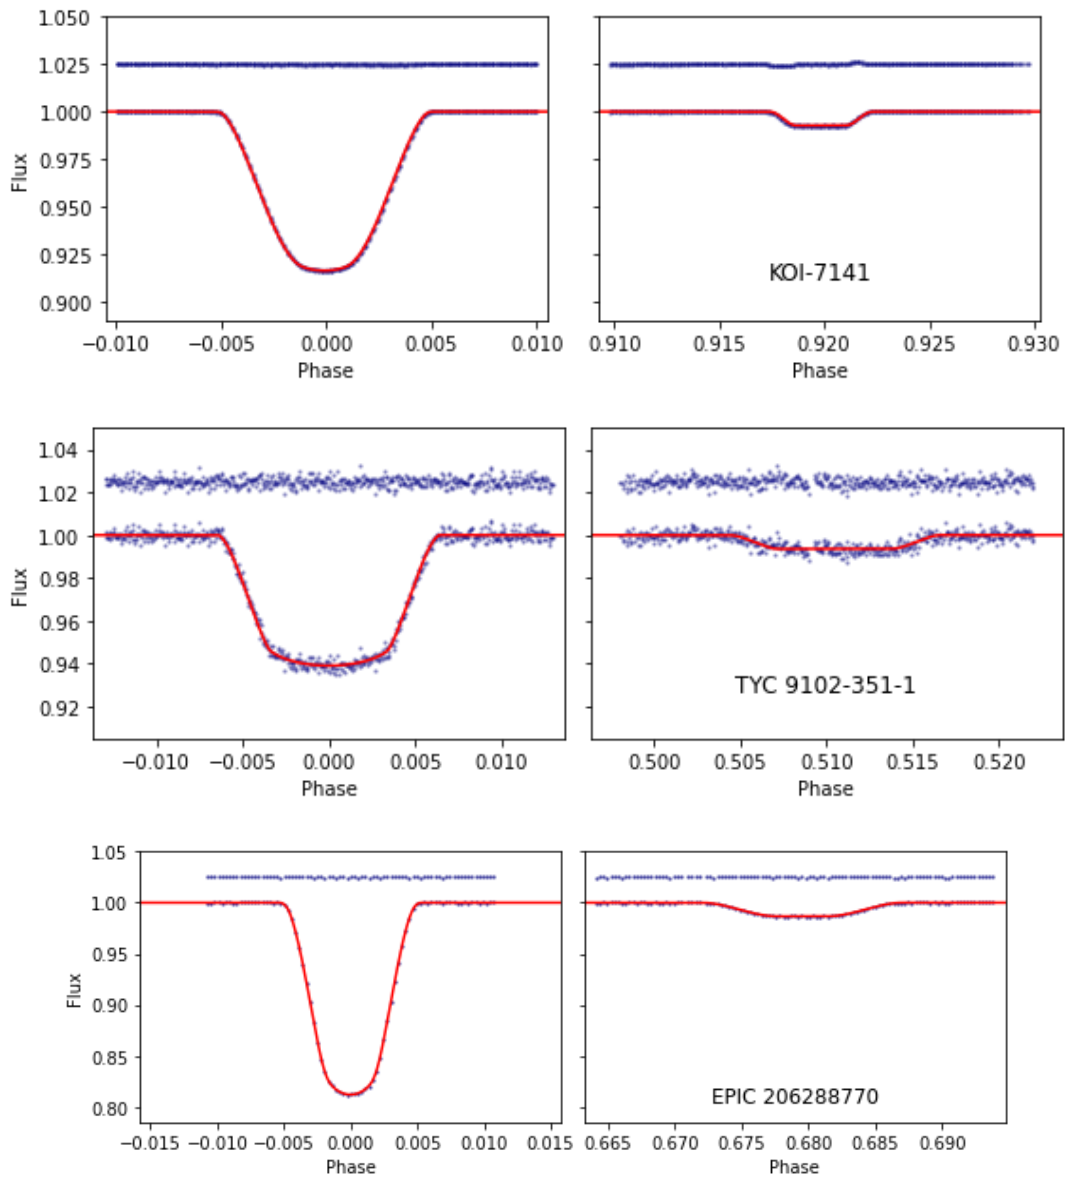

Supplement: Supplementary file 1 [file lcfits.pdf]
